# Supplementary material for: Combinatorial Selection with Costly Information
Source: arXiv:2412.03860 source file (2025-07-24)
Supplement: Supplementary file 1 [file appendix_continuous.tex]

\section{The Continuous Setting}\label{app:contin}

In this section, we describe how our entire framework extends to continuous settings. Our definitions of a Costly Information MDP and a CICS instance remain unchanged; now, for each state $s\in S$ of the MDP the action set $A(s)$ is allowed to be continuous, and so are the distributions $\dist(s, a, \cdot)$ for any action $a\in A(s)$. The only condition we require is that our MDPs will have a finite horizon $H$; this ensures that after a finite number of steps, our MDPs will reach a terminal state with probability $1$. We will discuss only the matroid-min-CICS setting; all the results extend to maximization and more general combinatorial settings as we have already discussed in~\Cref{app:maxim} and~\Cref{app:combinatorial} respectively.

\paragraph{Water Filling Amortization.} For a Markov chain $\mc=(S, \sigma, A, c, \dist, V, T)$, the water filling surrogate cost $W^*_\mc$ an be defined in the same bottom-up manner as in the discrete setting. In particular, for each state $s\in S$, we use $\mc_s$ to denote the sub-chain of $\mc$ that starts at state $s$. For terminal states $t\in T$, we have that $W^*_{\mc_t}= v(t)$. For non-terminal states $s\in S\setminus T$, we can recursively define the surrogate costs as
\[ W^*_{\mc_s} := \max\{Z_s,g_s\}\]
where $Z_s$ is the random variable corresponding to sampling a state $s'$ from distribution $\dist(s,a(s),\cdot)$\footnote{We use $a(s)$ to denote the unique action available at state $s$ in Markov chain $\mc$.} and then sampling from $W^*_{\mc_{s'}}$ and $g_s$ is the solution to equation
\[c(a(s)) = \expect{(g_s - Z_s)^+}.\]
Note that $W^*_\mc := W^*_{\mc_\sigma}$; the finite horizon assumption allows us to define these surrogate costs. Using the same arguments as in~\Cref{thm:MC-opt}, we can establish that the water filling index policy will be optimal for any instance of matroid-min-CICS over Markov chains.

Through the surrogate costs, we can write the optimality curve of a Markov chain $\mc$ as
\[f_{\mc}(y) = \expect{\min\{y, W^*_\mc\}}\]
and we can extend this definitions to arbitrary MDPs. From this, and by using a continuous (non-constructive) version of the second order stochastic dominance lemma, we can establish that the lower bound of~\Cref{thm:MDP-lb} holds in the continuous setting.

\paragraph{Local Approximation.} The definition of local approximation transfers as is in the continuous setting and so does our main composition theorem (\Cref{thm:la-comp}); the proof remains unchanged as at no point did we use the fact that the setting was discrete.

\textcolor{red}{Say that if $X$ is continuous, we can discretize it to an $\epsilon$-grid in order to enforce finite horizon, eg in the WS problem. Since the values depends on $X$, this can only cause as an $O(\epsilon)$ loss}
